# Supplementary material for: Interacting contagions are indistinguishable from social reinforcement
Source: arXiv:1906.01147 ancillary file (2019-06-04)
Supplement: Supplementary file 1 [file LHD18_ComplexCoinfection_SM.pdf]

# Interacting contagions are indistinguishable from social reinforcement
# Supplementary Material

Laurent Hébert-Dufresne,[1,2,3] Samuel V. Scarpino,[4,5,6,7,8] and Jean-Gabriel Young[9]

[1]*Vermont Complex Systems Center, University of Vermont, Burlington, VT 05405, USA*
[2]*Department of Computer Science, University of Vermont, Burlington, VT 05405, USA*
[3]*Département de physique, de génie physique et d'optique, Université Laval, Québec (Québec), Canada G1V 0A6*
[4]*Network Science Institute, Northeastern University, Boston, MA 02115, USA*
[5]*Marine & Environmental Sciences, Northeastern University, Boston, MA 02115, USA*
[6]*Physics, Northeastern University, Boston, MA 02115, USA*
[7]*Health Sciences, Northeastern University, Boston, MA 02115, USA*
[8]*ISI Foundation, 10126 Turin, Italy*
[9]*Center for the Study of Complex Systems, University of Michigan, Ann Arbor, MI 48109, USA*

## CONTENTS

I. Simulations of contagion models on contact networks 2

II. Inferring the complex contagion function 3
A. Inference under perfect conditions 3
B. Inference under noisy conditions 4
1. Bayesian inference: Likelihood 5
2. Bayesian inference: Posterior distribution 5
3. Bayesian inference: Priors 6
4. Data normalization 6
5. Model summary 7
6. Inference algorithm and diagnosis 7
7. Validation 8
C. Computational details 8
1. Supplementary Material figures 8
2. Figure 3 8

References 8

## I. SIMULATIONS OF CONTAGION MODELS ON CONTACT NETWORKS

To simulate all contagion models, we use a discrete time process with transmission and recovery probabilities $p_t$ and $p_r$ lesser than $10^{-3}$ to mimic the continuous time process used in our ODEs. At every time step, a contact between an infectious and susceptible node can transmit the contagion with probability $p_t$ and infectious nodes can recover with probability $p_r$. In all simulations, we initiate the system by infecting a random fraction $10^{-3}$ of nodes with the simple contagion, the complex contagion, or both interacting contagions.

All simulations take place on two simple network topologies: clustered network structures and equivalent random networks. Clustered networks are obtained by assigning every node to a number $m$ of cliques of size $n$, with an additional number $k$ of random neighbors. Equivalent random networks are obtained by keeping the same degree sequence but randomizing every connection to destroy cliques and reduce clustering close to zero. As discussed in the main text, we use regular networks where all nodes have the same degree to avoid conflicting the role of clustering with that of degree correlations.

The results of our simulations reported in the main text concern the global fraction of infected nodes at a given time (prevalence), number of new infections since the last observation (incidence) and local state correlations around infection events. To summarize the results shown in the main text, even though we parametrized all simulations to have a similar prevalence after 5000 time steps, complex and interacting contagions are more spatially correlated and therefore benefit from network clustering; all of these results can be used in practice to distinguish complex and interacting contagions from simple contagions, but not from each other. Additionally to the results shown in the main text, we find similar results for the number of infectious neighbours of individuals upon recovery. Indeed, on clustered networks, that number increases to 145% (median, 50% CI [130%,160%]) that of random networks for simple contagions, and 188% (median, 50% CI [166% 213%]) and 180% (median, 50% CI [144% 205%]) for interacting and complex contagions, respectively.

## II. INFERRING THE COMPLEX CONTAGION FUNCTION

The result of large scale epidemiological surveillance efforts are typically reported as times series $Y_{1:T} := (Y_1, Y_2, ..., Y_T)$ of the number of infected or newly infected individuals in a monitored populations. One may think of these time series as coarse-grained observations of some detailed spreading process, taking place on hidden contact networks. We now obtain a principled inference procedure to determine the parameters of the spreading processes, from the coarse grained time series alone (assuming that the family of possible contact networks is known).

For the sake of concreteness, we will hereafter assume that the spreading process is a complex Susceptible-Infected-Recovered (SIR) dynamics, and model the population as well-mixed, but the principles derived apply more broadly. The complex SIR dynamics is defined as one where nodes in the infectious state recover at a constant rate $\gamma > 0$ (i.e. transition from $I$ to $R$), but where susceptible individuals ($S$) get infected at a rate $\beta(I)$ that is a function of the density of infected individuals, in the neighbourhood of infected individuals. In a well-mixed population, these densities are governed by the mean-field system:

$$\frac{d}{dt}S(t) = -\beta\big(I(t)\big)I(t)S(t) \tag{1a}$$

$$\frac{d}{dt}I(t) = \beta\big(I(t)\big)I(t)S(t) - \gamma I(t) \tag{1b}$$

$$\frac{d}{dt}R(t) = \gamma I(t) \tag{1c}$$

There are no known closed form solutions, but it is fairly straightforward to generate time series by integrating from some initial condition $(S_0, I_0, R_0)$.

As is argued in the main text, this variable infection rate $\beta(I)$ helps capture exogenous processes such as social reinforcement and disease interactions. Our inference goal will be to determine $(\gamma, \beta(I))$.

### A. Inference under perfect conditions

If we get to observe the output of the mean-field dynamics at an infinite time-resolution, without any noise or misspecification whatsoever, the inverse problem of determining $\big(\gamma, \beta(I)\big)$ can be solved exactly, without much difficulties. We compute the empirical derivatives $\big(\hat{\dot{S}}(t), \hat{\dot{I}}(t), \hat{\dot{R}}(t)\big)$ of the time series, and invert Eqs. (1) to get the estimators:

$$\hat{\beta}(t) = \frac{-\hat{\dot{S}}(t)}{I(t)S(t)} \ , \tag{2a}$$

$$\hat{\gamma}(t) = \frac{\hat{\dot{R}}(t)}{I(t)} \ . \tag{2b}$$

Because the time series are directly generated by the dynamics appearing in Eq. (1), $\hat{\gamma}(t)$ does not actually depend on time, and will therefore be a constant. Any pair $(\hat{\dot{R}}(\tau), I(\tau))$ at some time $\tau$ is enough to evaluate the rate $\gamma$, although checking many pairs can in practice help average numerical errors out. In contrast, we expect $\hat{\beta}(t)$ to change with $t$, but only because density of infected individuals also varies with time. Making this dependency explicit yields

$$\hat{\beta}\big(I(t)\big) = \frac{-\hat{\dot{S}}\big(I(t)\big)}{I(t)\big(I(t)\big)} \ , \tag{3}$$

which gives a prescription for computing $\beta(I)$ exactly. Figure 1 confirms that the procedure works for various combinations of rates $\big(\gamma, \beta(I)\big)$.

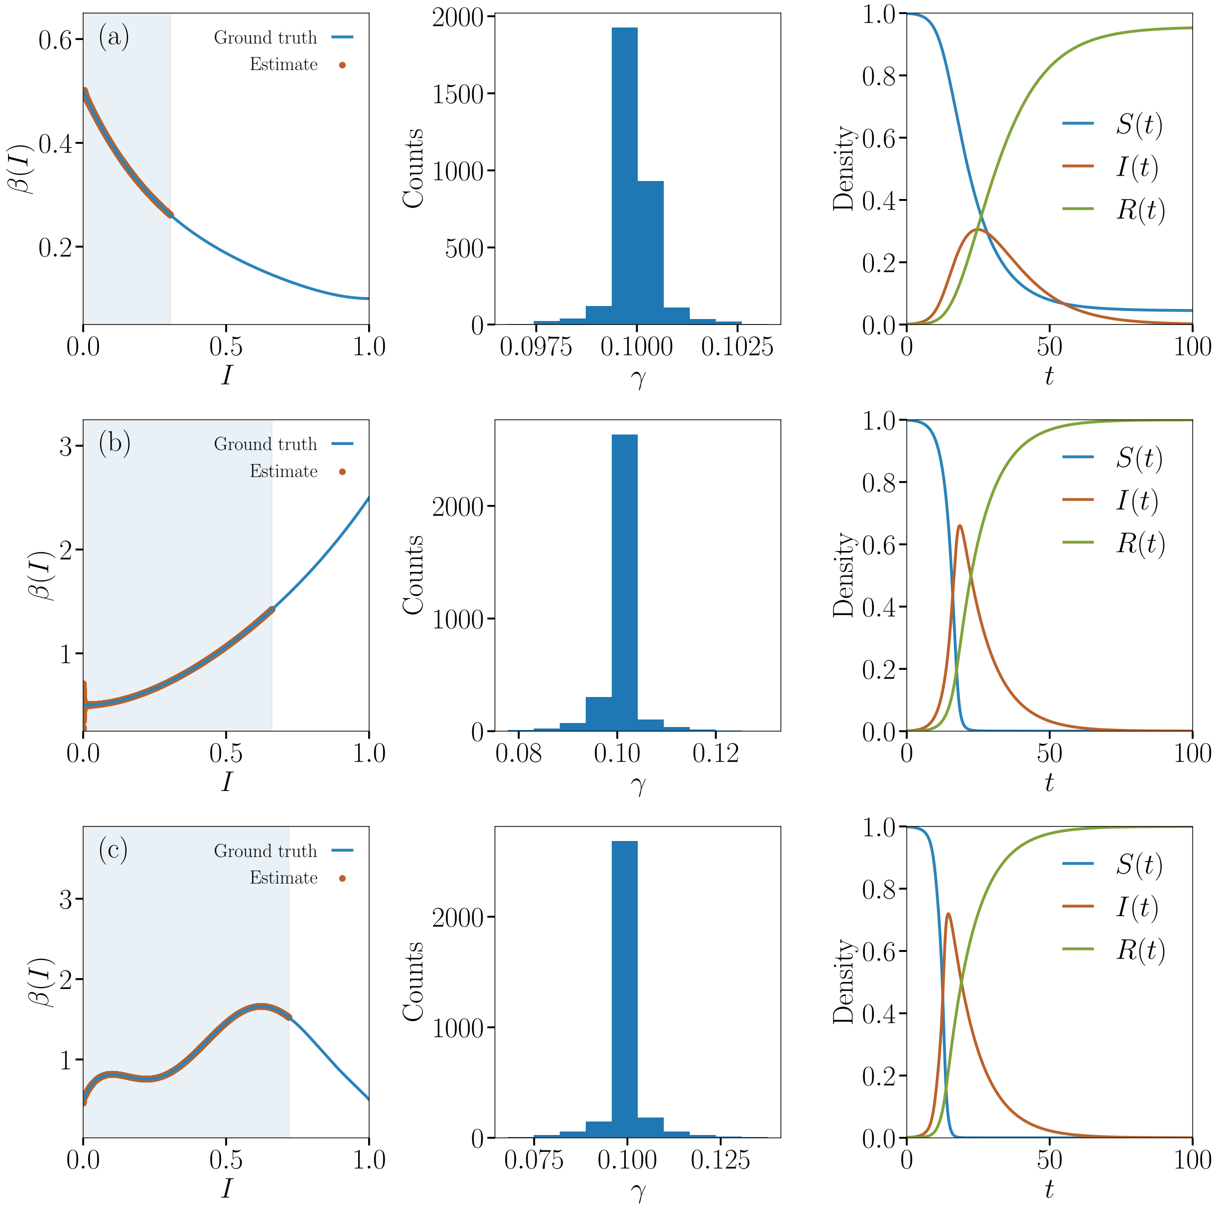


FIG. 1. **Inference under perfect conditions.** Inferred complex contagion function $\beta(I)$ (left column) and distribution of inferred recovery rate (central column) computed from time series generated by Eqs. (1), starting from the initial condition $(S_0, I_0, R_0 = (1-\varepsilon, \varepsilon, 0)$ with $\varepsilon = 0.001$ with $\gamma = 0.1$ and various functions $\beta(I)$. Note that it is only possible to infer the function $\beta(I)$ for observed values of $I$, indicated by a shaded region in the left column. The tested functions are *(a)* a decelerating contagion, *(b)* an accelerating contagion, and *(c)* some complicated contagion function with valleys and peaks.

## B. Inference under noisy conditions

Real epidemiological time series are noisier, less time-resolved, and often not as high dimensional[1] than the ones considered in Sec. II A. As a result, applying the inversion procedure of Eqs. (2) blindly to these series would seriously overfit the data. A more principled approach is needed to handle real datasets.

---

[1] We do not typically have—even noisy—measurements of $S(t)$ and $R(t)$.

### 1. *Bayesian inference: Likelihood*

We model the observed series as an imperfect and partial measurement of the macroscopic state of a detailed spreading process. That is, we assume that the detailed configuration $X_t \in \mathcal{X}$ of susceptible, infected and recovered individuals at time $t$ is measured only through a macroscopic quantity. We will consider two macroscopic measurements: (1) the density of infected individuals or prevalence, a real number in $[0, 1]$ which we will denote $Y_t$ to emphasize that the measurement is noisy and different from $I(t)$; and (2) the number of newly infected individuals or incidence, an integer in $[0, n]$ where $n$ is the population size. We will denote the incidence between time $t-1$ and $t$ as $Z_t$. The well-mixed assumption is translated by a population structure drawn from the Erdős-Rényi-Gilbert model of density $\rho \in [0, 1]$.

**Model for prevalence measurements.** The likelihood of the time series $Y_{1:T}$ is given by

$$P(Y_{1:T}|\beta,\sigma,\gamma,\rho,x_0) = \sum_G \int_{\mathcal{X}^T} P(Y_{1:T}|x_{1:T},\sigma)P(x_{1:T}|G,\beta,\gamma,x_0)P(G|\rho)dx_{1:T} \ . \tag{4}$$

where the integral is over all sequences of hidden states starting at $x_0 \in \mathcal{X}$, where $P(G|\rho)$ is a distribution over possible population structures parametrized by the density $\rho$, and where

$$P(Y_{1:T}|x_{1:T},\sigma) = \prod_t q(Y_t|I[x_t],\sigma) \tag{5}$$

is the noise component of the model, with $I[\cdot]$ the density of infected individuals in configuration $x_t \in \mathcal{X}$, and $q(Y|\mu,\sigma)$ the p.d.f. of the normal distribution of mean $\mu$ and standard deviation $\sigma$.

If we could compute Eq. (4) exactly in closed form, then we could compute the posterior distribution easily, and make inference on the parameters of the model. But both the sum over graphs and the integral over hidden states turn out to be complicated in all but the simplest cases (e.g., when the dynamics occurs on the fully connected population $\rho = 1$, with no noise). We must therefore resort to approximations. Noting that only the density of infected matters in Eq. (5), we approximate the integrals over states by their largest contribution, the mean-field solutions of Eqs. (1). This leads to

$$P(Y_{1:T}|\beta,\gamma,\rho,\sigma,y_0) = \prod_{t\in\tau_{\text{obs}}} q(Y_t|\tilde{y}_t(\beta,\gamma,\rho;y_0),\sigma) \ , \tag{6}$$

where $\tau_{\text{obs}}$ is the set of time steps for which we have an observation, and where $\tilde{y}_{1:T}(\beta,\gamma,\rho;y_0)$ is a time series of infectious density, given as the solution of Eq. (1) integrated from the initial condition $y_0 = (S_0, I_0, R_0)$.

**Model for incidence measurements.** In most real epidemics, we do not get to measure the density of infected. Instead, we often measure an incidence rate, e.g., the number new cases in a week. It turns out that we can carry out the inference highlighted above, with little modifications. We denote the time series of average incidence rate as $Z_{1:T}$. In the mean-field system of Eqs. (1) the number of new infected between times $t$ and $t' > t$ is $n[S(t) - S(t')]$ where $n$ is the population (assumed constant). Let us denote by $\tilde{z}_{1:T}(\beta,\gamma,\rho,n;y_0)$ the time series of these differences, i.e.:

$$\tilde{z}_t(\beta,\gamma,\rho,n;y_0) = n\Big[\tilde{y}_t(\beta,\gamma,\rho,y_0) - \tilde{y}_{t+1}(\beta,\gamma,\rho;y_0)\Big] \ , \tag{7}$$

The likelihood of the time series $Z_{1:T}$ under a normal noise is then:

$$P(Z_{1:T}|\beta,\gamma,\rho,\sigma,y_0,n) = \prod_{t\in\tau_{\text{obs}}} q(Z_t|\tilde{z}_t(\beta,\gamma,\rho,n;y_0),\sigma) \ , \tag{8}$$

where $q$ is, again, the p.d.f. of the normal distribution.

### 2. *Bayesian inference: Posterior distribution*

For both time series, we can obtain a posterior distribution over parameters by adding priors on the parameters of the likelihood. For example, for $Y_{1:T}$, we get:

$$P(\beta,\gamma,\sigma,y_0|Y_{1:T}) = \frac{P(Y_{1:T}|\beta,\gamma,\sigma,y_0)P(\beta,\gamma,\sigma,y_0)}{P(Y_{1:T})} \ , \tag{9}$$

and a similar equation holds for $Z_{1:T}$. Note that we have removed the dependency on $\rho$ since the density of a well-mixed population only influences the relative timescale of events as far as the SIR dynamics is concerned—we can simply *impose* a timescale and ignore $\rho$.

### 3. Bayesian inference: Priors

We opt for simple independent priors. For the scale of the noise, we choose a half-Cauchy prior on $\sigma > 0$ (centered on 0). For the initial conditions of the mean-field equations, we place a uniform prior on $I_0 \in [0, I_{\max}]$ where $I_{\max}$ is a preset upper bound[2], and a uniform prior on $S_0$ that preserves the normalization $S_0 + I_0 + R_0 = 1$, namely $S_0|I_0 \sim \text{Unif}(0, I_0)$. For $\gamma$, we place a very weak truncated normal prior centered at 0 (where $P(\gamma) = 0$ for $\gamma < 0$). Note that since incidence is essentially a discretized derivative of $nS(t)$, the data does not fully identify $\gamma$ (see Eq. (1)). Too tight or too diffuse of a prior is likely to misguide inference in that case.

Placing a prior on $\beta$ requires that we parametrize the function first. In principle, complex contagion is defined for *any* function $\beta : [0, 1] \to [0, \infty)$. Hence, we would ideally like to consider as broad a family of functions $\beta$ as possible a priori. But we also need to be careful not to overfit the data with overly flexible functions. We find that low degree Bernstein polynomials are perfectly suited to our purpose.

A Bernstein polynomial $B_N(I; \boldsymbol{\xi})$ of degree $N$ is a linear combination of the basis polynomials

$$b_{\nu,N}(I) = \binom{N}{\nu} I^{\nu}(1 - I)^{N-\nu}, \tag{10}$$

with coefficients $\xi_\nu$,

$$B_N(I; \boldsymbol{\xi}) = \sum_{\nu=0}^{N} \xi_\nu b_{\nu,N}(I), \tag{11}$$

that maps $[0, 1]$ to $(-\infty, \infty)$ in general. If $\xi_\nu > 0 \, \forall \, \nu$ however, $B_N(I; \boldsymbol{\xi})$ is non-negative on $[0, 1]$. This makes the Bernstein polynomials of some fixed degree $N$ with non-negative coefficients an *almost* perfect parametrization of $\beta$, as $\beta(I) = B_N(I; \boldsymbol{\xi})$.

The only "problem" with the unaltered Bernstein polynomials is that they are defined on the domain $[0, 1]$, whereas the observed densities $I(t)$ usually stay close to 0, never reaching 1. The net consequence is that we do not get to observe enough data to determine $\beta(I)$ on its whole domain. In theory, this should be reflected by an uninformative posterior distribution past $\max Y_{1:T}$; but in practice, sampling / optimization procedures suffer from such an ill-determined posterior. Thus we instead parametrize $\beta(I)$ with *rescaled* Bernstein polynomials, by mapping the domain of the standard Bernstein polynomials (the unit interval) to $[-\alpha I_{\max}, I_{\max}(1 + \alpha)]$, where $\alpha$ is an overshoot parameter that extends the boundary of the function a little bit out of the allowed region for $I_0$[3].

We find that in practice, low degree polynomials strikes a good balance between expressiveness, computational complexity, and regularization. We choose $N = O(1)$ in all our experiments because the model gets harder to sample as $N$ increases, due to the appearance of local minima. To capture the fact that we expect simple contagion a priori, we parametrize the coefficient of $\beta$ as $\xi_i = \mu_\xi + \Delta_i$ where $\mu_\xi$ is a baseline infection rate and $\Delta_i$ is a deviation. If all the $\{\Delta_i\}$ are close to 0, then the contagion rate is basically flat. Conversely, large $\{\Delta_i\}$ lead to a non-constant contagion function.

We use a very weak half-normal prior centered at 0 for $\mu_\xi$, and a Cauchy prior of scale $\sigma_\Delta$ for all the deviations $\Delta_i$.

### 4. Data normalization

To simplify the choice of priors and streamline inference, we normalize every time series before we start making our analyses. Specifically, we rescale the time interval to $\tau \in [0, 1]$. The inferred values can be transformed back to the original timescale via

---

[2] We set $I_{\max} = \max Y_{1:T}$ when we have prevalence data, and use an arbitrary upper bound when we have incidence data, see Sec. II C below for details on the latter case. Note that because the prior probability is uniform on $[0, I_{\max}]$ and zero everywhere else, the posterior probability associated to values of $I_0$ outside of this range will also be 0. Therefore, with the incidence data, we verify that the initial condition of the latent time series $\tilde{y}$ never "saturates"'and reaches values close to the chosen $I_{\max}$ a posteriori.

[3] The same considerations as for $I_0$ apply. We verify that the inferred time series never "saturate" a posteriori

the transformation $\tau = t/t_{\max}$, where $t_{\max}$ is the original running time of the time series. This is due to the fact that the ODEs

$$\frac{d}{d\tau}S = -\beta(I)IS, \qquad \frac{d}{d\tau}I = \beta(I)IS - \gamma I,$$

and

$$\frac{d}{dt}S = -t_{\max}\beta(I)IS, \qquad \frac{d}{dt}I = t_{\max}\beta(I)IS - t_{\max}\gamma I$$

have the same solutions. We present the results in their natural timescales for the sake of easy interpretability.

### 5. *Model summary*

The full model for prevalence data is $Y_{1:T}$

$$\begin{aligned}
Y_t &\sim N(\tilde{y}_t, \sigma^2) && t = 1, ..., T\\
\sigma^2 &\sim \text{Half-Cauchy}(0, \sigma_n)\\
\tilde{y}_{1:t} &= \text{SIR}(\beta(\boldsymbol{\xi}_{1..N}, \alpha), y_0, \gamma)\\
I_0 &\sim \text{Unif}(0, I_{\max})\\
S_0|I_0 &\sim \text{Unif}(0, I_0)\\
\xi_i &= \mu_\xi + \Delta_i\\
\gamma &\sim \text{Half-Normal}(0, \sigma_\gamma^2)\\
\mu_\xi &\sim \text{Half-Normal}(0, \sigma_\mu^2)\\
\Delta_i &\sim \text{Cauchy}(0, \sigma_\Delta^2) && i = 0, ..., N
\end{aligned}$$

where $\text{SIR}(\beta(\boldsymbol{\xi}_{1..N}, \alpha), y_0, \gamma)$ returns a mean-field time series of prevalence with initial conditions $y_0 = (S_0, I_0, 1 - S_0 - I_0)$, recovery rate $\gamma$, and a contagion function $\beta$ parametrized by the degree $N$ Bernstein polynomials of coefficients $\boldsymbol{\xi}$. The full model for incidence data $Z_{1:T}$ is almost identical, with the differences:

$$\begin{aligned}
Z_t &\sim N(\tilde{z}_t, \sigma^2) && t = 1, ..., T\\
\tilde{z}_t &= n(\tilde{y}_t - \tilde{y}_{t+1})\\
\gamma &\sim \text{Normal}(\mu_\gamma, \sigma_\gamma^2)
\end{aligned}$$

where $n$ is a population size given a priori, $\mu_\gamma$ is used to inform the inference, and where $\gamma$ is constrained to $\mathbb{R}^+$.

### 6. *Inference algorithm and diagnosis*

We approximate the posterior distribution with samples generated by an Hamiltonian Monte-Carlo (HMC) sampler. This process can be carried out automatically by implementing the model[4] in the `STAN` probabilistic programming language [1].

There are a number of post-sampling check that allows one to verify whether HMC samples are well behaved [1]. Of all the possible diagnostics, the presence of divergent transitions is the most important one: It indicates whether there are regions of the posterior that are hard to sample due to high curvature. When we use Bernstein polynomials of a high degree $N$, the posterior tends to become multimodal—even though one of the modes dominates the others. Divergent transition, can happen as a result of this peculiar geometry. To see why, consider a highly non-linear ground truth $\beta(I)$. There are at least two "explanations" of the data, and they are separated by steep chasms: A flat averaged out $\beta(I)$ with significant noise $\sigma^2$, and a posterior close to the ground-truth with next to no noise $\sigma^2$. We avoid the divergent transitions brought about by this geometry by (a) sticking to relatively low order polynomials, and (b) running long burn-in periods to make sure that the divergent transitions encountered

[4] Our implementation is available online `https://www.github.com/jg-you/complex-coinfection-inference/`.

on the way to the dominant mode do not pollute our inference. Note, however, that some unavoidable divergent transitions occur when the data determines the model extremely well—i.e., when the data is measured without noise—such that any description of the data but the best is a comparatively bad one. These can be safely ignored.

#### 7. *Validation*

In Figs. 2–6, we investigate the performance of the inference method by generating artificial data with the model itself.

Figure 2 shows noisy time series, sampled more or less frequently. Even when most data points are absent, the posterior distribution correctly captures the shape of the function $\beta(I)$. Importantly, point estimates are not as accurate in recovering the contagion function as the full distribution; sampling is not only useful, and it is necessary.

Figure 3 shows noisy time series, under various level of noise $\sigma^2$. When there is no noise, even a sparse time series is enough to perfectly reconstruct the time series. Furthermore, reconstruction remains qualitatively possible under large level of noise.

Figures 4 and 5 show the effect of prior misspecification on inference with incidence data. Imprecise but vague prior tend to yield good results (Fig. 4). While precise but incorrect priors, lead to bad results (Fig. 5) This shows that incidence partially identifies $\gamma$, and suggest that we are better off using vague priors when dealing with real data.

Figure 6 shows the inference we would have made, had we kept only a (random) fraction of all the Monte Carlo samples. The figure tells us that only a few samples are really necessary.

### C. Computational details

In all experiments (main text and SM alike), we set the scale of the prior on the noise to $\sigma_n = 1$ and the scale of the prior on the deviations $\{\Delta_i\}$ to $\sigma_\Delta = 1$. When we deal with prevalence data, we set the scale of the prior on $\gamma$ to $\sigma_\gamma = 100$, and the overshoot parameter $\alpha$ on the range of $\beta$ to $\alpha = 0.1$. When we deal with incidence data, we set a case specific prior for $\gamma$ (see below) and use no overshoot $(\alpha = 0)$ because the prevalence time series is latent in the first place.

The other parameters are varied from experiments to experiments[5].

#### 1. *Supplementary Material figures*

In all SM figures, we use polynomials of degree $N = 8$, and a scale parameter $\sigma_\mu = 100$. When dealing with incidence data, we use a tight prior on $\gamma$ with $\mu_\gamma = \tilde{\gamma}$ and $\sigma_\gamma = 0.1$ (where $\tilde{\gamma} = 0.1$ is the ground-truth), except in Figs. 4–5 where we intentionally give a bad prior. The population size is always set to its true value, $n = 100\,000$.

For most experiments shown in the Supplementary Materials, we make our inference using 4 chains of 500 samples, all initialized with a burn-in period of 500 iterations. In figure 3, however, we use shorter chains when the data determines the posterior very well. Specifically, for an artificial noise level of $\sigma^2 = 0$, we only use 100 warm-up iterations and 100 samples per chains. For an artificial noise level of $\sigma^2 = 0.01$, we use 250 warm-up iterations and 250 samples per chains.

#### 2. *Figure 3*

In Figure 3 of the main text, we use polynomials of degree $N = 6$, and a scale parameter $\sigma_\mu = 100$. The population size is set to its true value, $n = 10\,000$. We make our inference using 4 chains of 1000 samples, all initialized with a burn-in period of 1000 iterations. The true recovery rate is given as a prior with noise $\sigma_\gamma = 1$ for the fit on incidence data.

[1] B. Carpenter, A. Gelman, M. D. Hoffman, D. Lee, B. Goodrich, M. Betancourt, M. Brubaker, J. Guo, P. Li, and A. Riddell, Journal of Statistical Software **76** (2017).
[2] J.-G. Young, URL https://github.com/jg-you/complex-coinfection-inference/.

[5] Note that all of the details below are also available in our replication files, see Ref. [2].

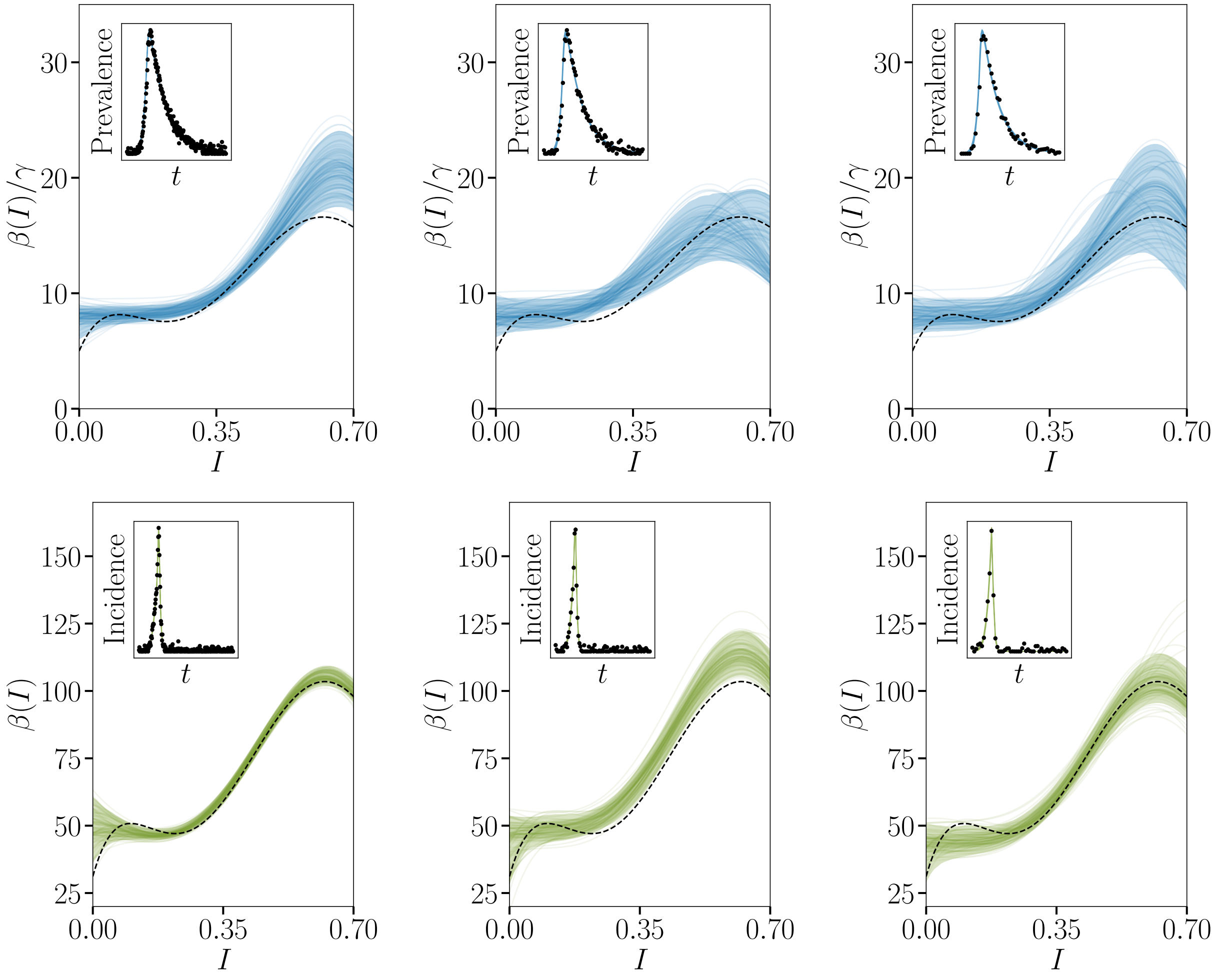


FIG. 2. **Inference at different levels of sampling.** (top row) Inference on prevalence data. (bottom row) Inference on incidence data. We use a population size of $n = 100\,000$. In all cases, the same base time series is used. It is generated with Eqs. (1) using $\gamma = 0.1$, $(S_0, I_0, R_0 = (1-\varepsilon, \varepsilon, 0)$ where $\varepsilon = 0.001$, and the complicated $\beta(I)$ function shown as the ground-truth in the main plot. We keep (from left to right): $T = 250$, $T = 100$ and $T = 50$ regularly spaced data points. An independent Gaussian noise of variance $\sigma^2 = 0.2$ is applied to the prevalence measurements, while the variance is set to $\sigma^2 = 2 \times n \times T$ for the incidence measurements. The resulting series are shown in the inset, alongside a posterior fit (95% of the a posteriori incidence curves). The main plots show the inference results for the three level of data sparsity. The ground truth is shown with a dotted line, alongside with 95% of the data (shaded region), and 100 random posterior samples to emphasize sample-to-sample variability.

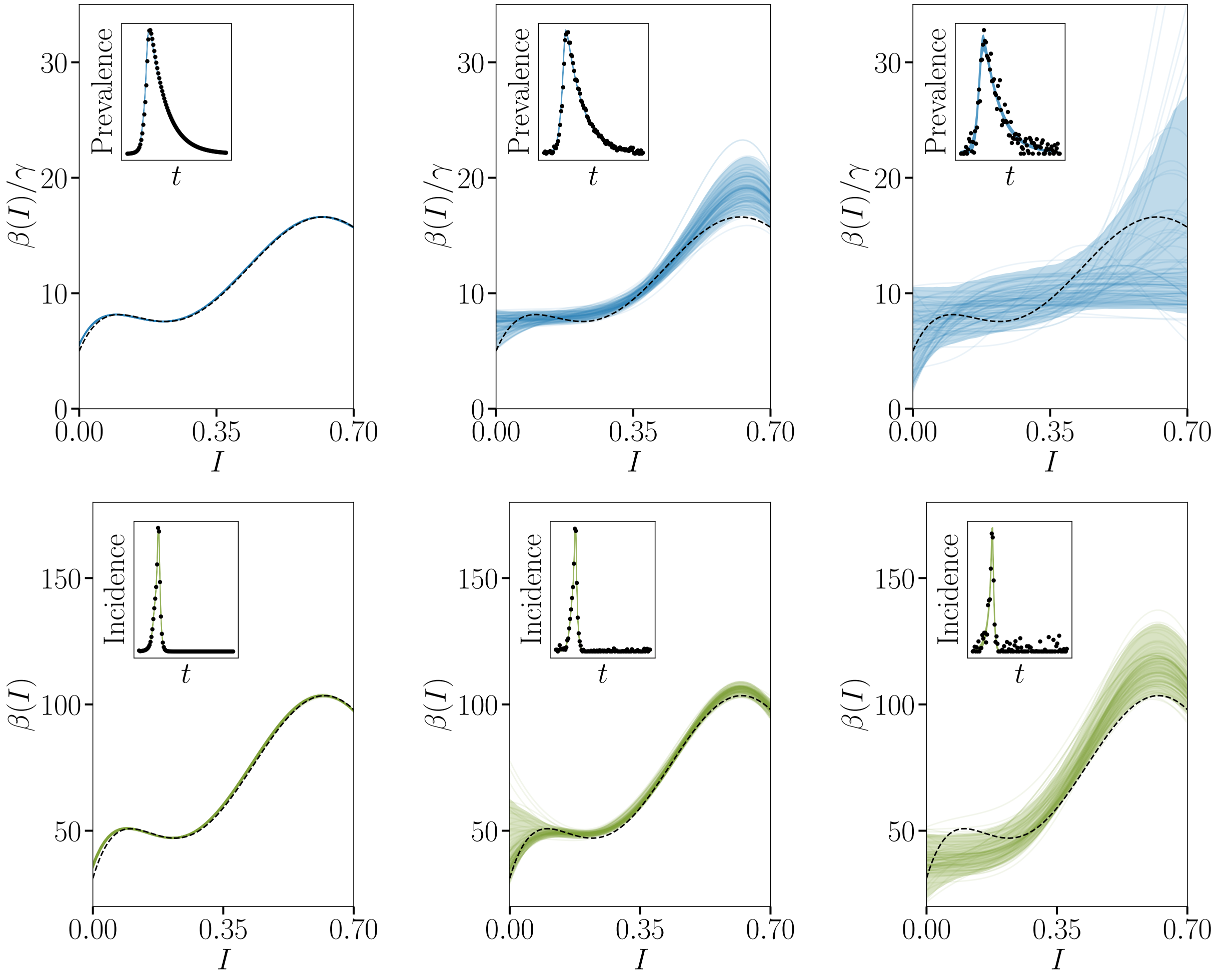


FIG. 3. **Inference at different levels of noise.** See the caption of 2 for how to read this figure. The artificial time series are obtained by sampling the latent time series at $T = 100$ regularly spaced points. An independent Gaussian noise of variance (from left-to-right) $\sigma^2 = 0, 0.1$ and $0.5$ is applied to the prevalence measurements. The variance is set to $10 \times \sigma^2 \times n \times T$ for the incidence measurements.

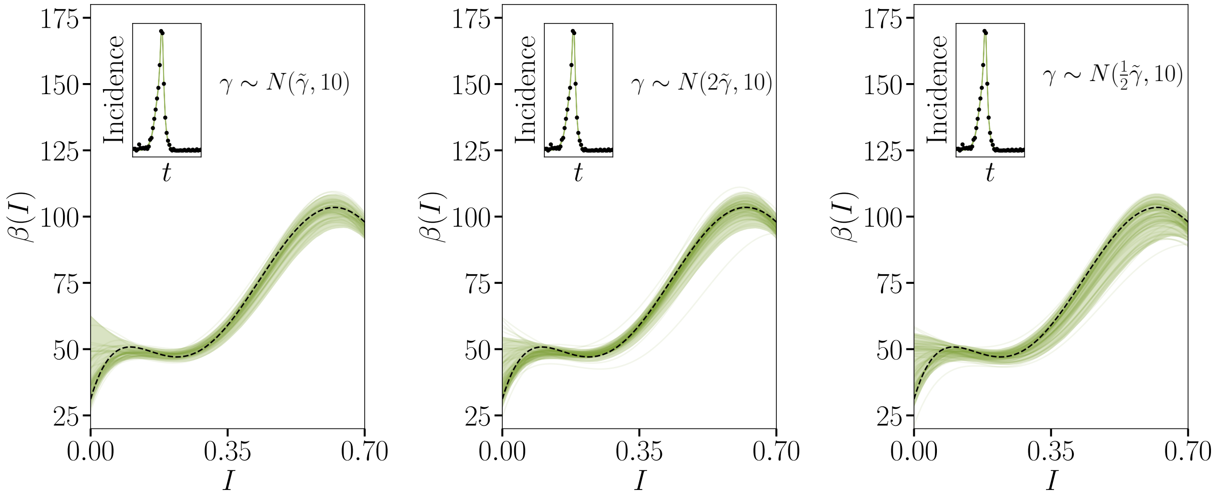


FIG. 4. **Inference with incidence data and vague imprecise priors.** See the caption of 2 for how to read this figure. The ground-truth is $\tilde{\gamma} = 0.1 t_{\max}$ where $t_{\max} \approx 7$ is a constant introduced in the data normalization step (see Sec. II B 4). In the 3 cases shown, the location of the prior on $\gamma$ is inaccurate, but the the variance is comparatively large.

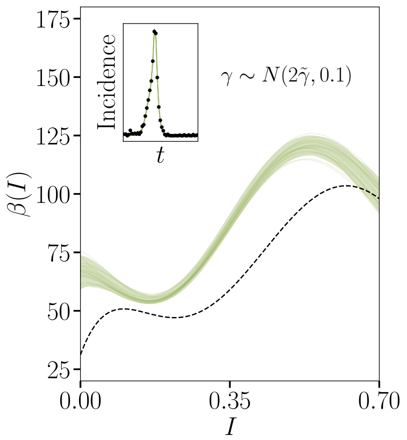


FIG. 5. **Inference with incidence data and tight imprecise priors.** Same experiment as a in Fig. 4, but this time we use a much narrower prior. The posterior moves away from the ground-truth. In the case shown, the infection rate is shifted to compensate for the increased infection rate, leaving the a posteriori incidence curves basically unaltered.

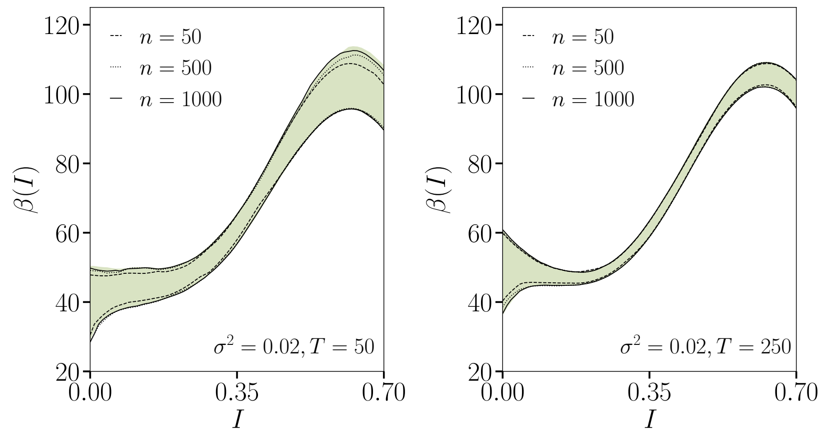


FIG. 6. **Impact of the number of samples.** Regions covered by 95% of the posterior draws, when $n$ samples are used, for two different levels of temporal sampling $T$. The shaded regions shows this range for $n = 2000$ samples (the actual number of sample used in all our experiments). Even for temporally sparse data ($T = 50$), a few samples suffice to determine the confidence interval.
